# Supplementary material for: Pix2Video: Video Editing using Image Diffusion
Source: arXiv:2303.12688 source file (2023-03-22)
Supplement: Supplementary file 1 [file appendix.tex]

% \appendix

% \section{...}

% TODO
